# Supplementary material for: RT-GS2: Real-Time Generalizable Semantic Segmentation for 3D Gaussian Representations of Radiance Fields
Source: arXiv:2405.18033 source file (2024-08-30)
Supplement: Supplementary file 1 [file pseudocode.tex]

\section{Pseudocode}

We present an overview of the method by 

\begin{algorithm}
\caption{Train view independent features}
\For{each scene k}
\State G^k$ \gets train\_gaussian\_splatting\_representations($p^k$, $I^k$)
\EndFor

\For{each scene k}
    \For{m in \{$p^k_1, p^k_1, p^k_1, ...$\}}
        \For{n in \{$p^k_1, p^k_1, p^k_1, ...$\}}
            \State $fr_m$ \gets compute\_frustrum(m) $
            \State $fr_n$ \gets compute\_frustrum(n) $
            \If {overlap($fr_m$, $fr_n$)}
                \State $g_m^k$ \gets ($x_m^k, \Sigma_m^k, \alpha_m^k, c_m^k$)
                \State $g_n^k$ \gets ($x_n^k, \Sigma_n^k, \alpha_n^k, c_n^k$)
                \State $f_m^k$ \gets PointTransformerV3($g_m^k$)
                \State $f_n^k$ \gets PointTransformerV3($g_m^k$)
                \State $loss$ \gets \(L_{cl}\)($f_m^k$, $f_n^k$)
            \EndIf
        \EndFor
    \EndFor
\EndFor
\end{algorithm}

\begin{algorithm}
\caption{View-dependent / View-independent fusion}
\For{each scene k}
    \State $f^k$ \gets PointTransformerV3($G^k$)
    \For{each pose $p^k$ of $G^k$}
        \State \(\hat{\mathbf{I}}^k_j, \mathbf{Z}^k_j\) \gets render\_by\_splatting($G^k$, $f^k$)
        \State \(\hat{\mathbf{S}}^k_j\) \gets \(Dec(\psi(Enc_{VD}(\hat{\mathbf{I}}^k_j), Enc_{VI}(\mathbf{Z}^k_j, \hat{\mathbf{I}}^k_j)))\)
        \State loss \gets \(L_{sem}\)(\(\hat{\mathbf{S}}^k_j, \mathbf{S}^k_j\))
    \EndFor
\EndFor
\end{algorithm}

\begin{algorithm}
\caption{Test}
\For{each scene k}
    \State $f^k$ \gets PointTransformerV3($G^k$)
    \For{each pose $p^k$ of $G^k$}
        \State \(\hat{\mathbf{I}}^k_j, \mathbf{Z}^k_j\) \gets render\_by\_splatting($G^k$, $f^k$)
        \State \(\hat{\mathbf{S}}^k_j\) \gets \(Dec(\psi(Enc_{VD}(\hat{\mathbf{I}}^k_j), Enc_{VI}(\mathbf{Z}^k_j, \hat{\mathbf{I}}^k_j)))\)
    \EndFor
\EndFor
\end{algorithm}
